# Supplementary material for: Particle Semi-Implicit Variational Inference
Source: arXiv:2407.00649 source file (2025-01-14)
Supplement: Supplementary file 1 [file assumptions2.tex]

\section{On \Cref{ass:coupling_and_base,ass:p_bounded_n_lip_model,ass:q_l_b}}

We shall show that the Gaussian kernel $k_\theta(x|z) = \cal{N}(x;\mu_\theta(z), \rm{Diag}(\sigma_\theta^2(z)) I_{d_x})$,i.e.,
$$
k_\theta(x|z) = \frac{1}{(2\pi)^{d_x/2}\prod_{i=1}^{d_x}\sigma_\theta(z)_i} \exp \left( -\frac{1}{2} (x - \mu_\theta(z))^T (\rm{Diag}(\sigma_\theta^2(z))I_{d_x})^{-1}(x - \mu_\theta(z)) \right),
$$
where $\mu_\theta : \r^{d_z} \mapsto \r^{d_x}$ and $\sigma_\theta: \r^{d_z} \mapsto \r^{d_x}_{>0}$, satisfies \Cref{ass:q_l_b,ass:coupling_and_base} under some regularity assumptions on $\mu_\theta$ and $\sigma_\theta$:
\begin{assumption}[$\mu_\theta$ and $\sigma_\theta$ are bouneded.]
\label{ass:mu_siga_bounded2}
 $\mu$ and $\sigma$ are bounded, i.e., there exists constants $B_\sigma, B_\mu, L_\sigma \in \bb{R}_{>0}$ such that the following holds for all $(\theta, z) \in \Theta \times \z$:
	\begin{align*}
		\|\nabla_{(\theta, z)} \sigma_\theta(z)\|_F &\le B_\sigma, \\
		\|\nabla_{(\theta, z)}\mu_\theta(z)\|_F &\le B_\mu, \\
		\|\sigma_\theta(z)\| &> L_\sigma.
	\end{align*}
\end{assumption}
\begin{assumption}
	\label{ass:lip_mu_siga2}
	(Gradient Lipschitz)$\mu_\theta$ and $\sigma_\theta$ has Lipschitz gradient:
	\begin{align*}
		\|\mu_\theta(z) - \mu_{\theta'}(z')\| &\le K_\mu \|(\theta, z) -  (\theta', z')\|, \\
		\|\sigma_\theta(z) - \sigma_{\theta'}(z')\| &\le K_\sigma \|(\theta, z) -  (\theta', z')\|.
	\end{align*}
\end{assumption}
\subsection{$k_\theta$ satisfies \Cref{ass:q_l_b}}

\textbf{Boundedness.} First, we shall show with $k_\theta$ is bounded. Clearly, we have $k_\theta \in \left [0, (2\pi)^{-d_x/2}\prod_{i=1}^{d_x}\sigma^{-1}_\theta(z)_i \right ]$ hence  $|k_\theta|$ is bounded from \Cref{ass:mu_siga_bounded2}. Now to show that the gradient is bounded $||\nabla_{(\theta, x, z)} k_\theta(x|z)||$, we have the following
%\adaml{Sorry, I started fiddling with this before realising it wasn't a finished argument---feel free to ignore/delete anything I've done that is unhelpful.}
%
\begin{align*}
\nabla_x k_\theta(x|z) &= k_\theta(x|z) \left ( \frac{x- \mu_\theta(z)}{\sigma_\theta^2(z)}\right ), \\
\nabla_z k_\theta(x|z) &= \nabla_z  \mu (z)\nabla_\mu  \cal{N}(x;\mu_\theta(z), \sigma^2_\theta(z)I_{d_x})  + \nabla_z \sigma_\theta (z) \nabla_\sigma \cal{N}(x;\mu_\theta(z), \sigma^2_\theta(z)I_{d_x}),  \\
\nabla_\theta k_\theta(x|z) &= \nabla_\theta  \mu (z)\nabla_\mu  \cal{N}(x;\mu_\theta(z), \sigma^2_\theta(z)I_{d_x})  + \nabla_\theta \sigma_\theta (z) \nabla_\sigma \cal{N}(x;\mu_\theta(z), \sigma^2_\theta(z)I_{d_x}).  \\
\end{align*}
Using the fact that
$$
\|\nabla_{(x,\mu, \sigma)}  \cal{N}(x;\mu_\theta(z), \sigma^2_\theta(z)I_{d_x})\| < \infty,
$$
and \Cref{ass:mu_siga_bounded2}, we obtain as desired.

\textbf{Lipschitz.} Recall that
\begin{align*}
	\nabla_{x} k_\theta(x|z) &= \nabla_x [\baseK(\phi^{-1}_\theta(z, x))\rm{det}(\nabla_{x} \phi^{-1}_\theta(z, x))] = \rm{det}(\nabla_{x} \phi^{-1}_\theta(z, x)) \nabla_x [\baseK\left ( \phi^{-1}_\theta(z, x)\right )]\\ 
	&= \left [ \prod_{i=1}^{d_x}{\sigma_\theta^{-1}(z)_i}\right ]\rm{Diag}(\sigma_\theta(z))^{-1} \nabla_x \baseK(\phi^{-1}_\theta(z, x))\\
	&=\tilde{\Sigma}^{-1}_\theta(z)\nabla_x \baseK(\phi^{-1}_\theta(z, x))
\end{align*}
where $\tilde{\Sigma}_\theta(z) := \Pi_{\theta}(z)\rm{Diag}(\sigma_\theta(z)),
$
and $\Pi_\theta(z) := \left  [\prod_{i=1}^{d_x}{\sigma_\theta(z)_i} \right ]$.
\begin{align*}
	&\|\nabla_{x} k_\theta(x|z) - \nabla_{x} k_{\theta'}(x'|z) \|\\
	&\le \|\tilde{\Sigma}^{-1}_\theta(z)\nabla_x \baseK(\phi^{-1}_\theta(z, x)) - \tilde{\Sigma}^{-1}_{\theta'}(z)\nabla_x\baseK(\phi^{-1}_\theta(z, x))\| \\
	&\le \|\tilde{\Sigma}^{-1}_\theta(z)\|_F \|\nabla_x\baseK(\phi^{-1}_{\theta}(z, x)) - \nabla_x\baseK(\phi^{-1}_{\theta'}(z', x))\| \\
	&+\|\tilde{\Sigma}^{-1}_\theta(z) - \tilde{\Sigma}^{-1}_{\theta'}(z')\|_F \|\nabla_x\baseK(\phi^{-1}_\theta(z, x))\|.
\end{align*}
using the fact that $\baseK$ is a standard Gaussian with bounded derivatives hence is Lipschitz and \Cref{prop:sigma_lipschitz}, we obtain 
\begin{align*}
	\|\nabla_{x} k_\theta(x|z) - \nabla_{x} k_{\theta'}(x'|z) \| &\le C \|\phi^{-1}_{\theta}(z, x)- \phi^{-1}_{\theta'}(z, x')\|\\
	&+ C\|(\theta, z)-(\theta',z')\| \\
	&\le C\|(\theta, z)-(\theta',z')\|.
\end{align*}
recall that $\phi^{-1}_{\theta}(z, x) = \frac{x - \mu_\theta(z)}{\sigma_\theta(z))}$
\begin{align*}
	\|\phi^{-1}_{\theta}(z, x)- \phi^{-1}_{\theta'}(z, x')\| &= \| \rm{Diag}(\sigma_\theta(z))^{-1}(x - \mu_\theta(z)) - \rm{Diag}(\sigma_{\theta'}(z'))^{-1}(x' - \mu_{\theta'}(z))\| \\
	&\le \|\rm{Diag}(\sigma_\theta(z))^{-1}\|_F \|(x,\mu_\theta(z))-(x',\mu_{\theta'}(z))\|\\
	&+ ...
\end{align*}
\jll{Unfortunately this part is where it falls apart...., we need the inverse map of $\phi$ to be Lipschitz which it does not seem to be.}

\begin{proposition}[$\Sigma_\theta^{-1}$ is Lipschitz and bounded]
	\label{prop:sigma_lipschitz}
	The map $\Sigma_\theta^{-1}$ is Lipschitz: there exists a constant $K_\Sigma \in \bb{R}_{>0}$ such that for all $(\theta,z), (\theta',z')\in \Theta \times \z$,
	$$
	\|\tilde{\Sigma}^{-1}_\theta(z) - \tilde{\Sigma}^{-1}_{\theta'}(z')\|_F\le K_\Sigma \|(\theta, z)-(\theta',z')\|.
	$$
\end{proposition}
\begin{proof}
	We begin with showing Lipschitz
	\begin{align*}
		\|\tilde{\Sigma}^{-1}_\theta(z) - \tilde{\Sigma}^{-1}_{\theta'}(z')\|_F &\le \|\Pi_\theta(z)^{-1}\sigma^{-1}_\theta(z)-\Pi_\theta'(z')^{-1}\sigma^{-1}_{\theta'}(z')\| \\
		&\le \left \|\frac{\Pi_\theta(z)\sigma_\theta(z) - \Pi_{\theta'}(z')\sigma_{\theta'}(z')}{\Pi_\theta(z)\sigma_\theta(z)\Pi_{\theta'}(z')\sigma_{\theta'}(z')}\right\|\\
		&\le  C \left \|{\Pi_\theta(z)\sigma_\theta(z) - \Pi_{\theta'}(z')\sigma_{\theta'}(z')}\right\|\\
		&\le C \left |\Pi_\theta(z) - \Pi_{\theta'}(z')\right |\|\sigma_\theta(z)\|\\
		&+ C |\Pi_\theta(z)|\left \|{\sigma_\theta(z) - \sigma_{\theta'}(z')}\right\|,
	\end{align*}
	where $C$ is a constant that changes at each line.
	using the fact $$|\Pi_\theta(z)-\Pi_\theta(z)|\le \sum_{i=1}^{d_x}|\sigma_{\theta}(z) - \sigma_{\theta'}(z')| \le \|\sigma_{\theta}(z) - \sigma_{\theta'}(z')\|_1\le \sqrt{d_x}\|\sigma_{\theta}(z) - \sigma_{\theta'}(z')\|$$
\end{proof}

\subsection{$k_\theta$ satisfies \Cref{ass:coupling_and_base}}
For $k_\theta$, one choice of coupling function and noise distribution is $\phi_\theta (z, \epsilon) = \sigma_\theta(z) \odot \epsilon + \mu_\theta(z)$ and $\baseK = \cal{N}(0,I_{d_x})$, where $\odot$ is element-wise product.

The gradient is given by
$$
\nabla_{(\theta, z)}\phi_\theta (z, \epsilon  ) : =  \nabla_{(\theta,z)} \sigma_\theta(z) \cdot  \rm{Diag}(\epsilon) + \nabla_{(\theta,z)} \mu_\theta(z),
$$
and hence $\|\nabla_{(\theta, z)}\phi_\theta (z, \epsilon  )\|_F \le \|\epsilon\|\|\nabla_{(\theta,z)} \sigma_\theta(z)\|_F + \|\nabla_{(\theta,z)} \mu_\theta(z)\|_F \le B_\sigma\|\epsilon \| + B_\mu$.
As for Lipschitz gradient property, we have
\begin{align*}
	\|\nabla_{(\theta, z)}\phi_\theta (z, \epsilon) - \nabla_{(\theta, z)}\phi_{\theta'} (z', \epsilon)\|
	&\le \|
		[\nabla_{(\theta,z)} \sigma_\theta(z) - \nabla_{(\theta,z)} \sigma_{\theta'}(z')] \cdot \rm{Diag}(\epsilon)\|_F\\
	&+ \|\nabla_{(\theta, z)} \mu_\theta(z)-  \nabla_{(\theta,z)} f_{\theta'}(z')\|_F\\
	&\le \|\nabla_{(\theta,z)} \sigma_\theta(z) - \nabla_{(\theta,z)} \sigma_{\theta'}(z')\|_F\|\epsilon \| \\
	&+ \|\nabla_{(\theta, z)} \mu_\theta(z)-  \nabla_{(\theta,z)} f_{\theta'}(z')\|_F, \\
	&\le \|\epsilon\|K_\sigma \|(\theta,z) - (\theta',z')\| + K_\mu \|(\theta,z) - (\theta',z')\| \\
	&\le  (K_\sigma \|\epsilon\|  + K_\mu)\|(\theta,z) - (\theta',z')\|
\end{align*}
where the desired result is obtained from the sub-multiplicative property of the Frobenius norm, and the Lipschitz gradient property of $\sigma_\theta(z)$ and $f_{\theta}(z)$, and $\epsilon$ is fixed and $\|\epsilon\|< \infty$.
