# Supplementary material for: Particle Semi-Implicit Variational Inference
Source: arXiv:2407.00649 source file (2025-01-14)
Supplement: Supplementary file 2 [file euler.tex]

\newcommand{\efl}{\cal{E}^\fudge_\lambda}
\newcommand{\thetaf}{\theta^\fudge}
\newcommand{\rf}{r^\fudge}
\subsection{Proposition of \Cref{prop:euler}}
\begin{proof}[Proposition of \Cref{prop:euler}]
\label{proof:discretization}
Consider the path
$$
\nu: t \mapsto (\thetaf_n - h t \nabla_\theta \efl(\thetaf_n, \rf_n), (\sf{id} - ht \nabla_z \delta_r \efl[\thetaf_n, \rf_n])_\#\rf_n ).
$$
Clearly, $\nu(1) = (\thetaf_{n+1}, \rf_{n+1})$; $\nu(0) = (\thetaf_{n}, \rf_{n})$; and
$$
\partial_t{\nu}(t) = (h \nabla_\theta \efl(\thetaf_n, \rf_n), h\nabla \cdot \left (\rf_n \nabla_z \delta_r \efl[\thetaf_n, \rf_n]\right )).
$$
For shorthand, we write $(\thetaf_{n+t}, \rf_{n+t}):=\nu(t)$. Thus, we can rewrite
\begin{align}
\label{eq:desired_result}
    \efl(\nu(1)) - \efl(\nu(0)) &= \frac{\rm{d}}{\rm{d}t}{\efl}(\nu(0)) + \int_0^1 \frac{\rm{d}}{\rm{d}t}[\efl(\nu(t)) - \efl(\nu(0))]\,\rm{d}t \nonumber \\
    &\le \frac{\rm{d}}{\rm{d}t}{\efl}(\nu(0)) + \int_0^1 \left |\frac{\rm{d}}{\rm{d}t}[\efl(\nu(t)) - \efl(\nu(0))]\right |\,\rm{d}t
\end{align}
For the first term, we have
$
\frac{\rm{d}}{\rm{d}t}{\efl}(\nu(0)) = - h\|\nabla \efl(\thetaf_{n}, \rf_{n})\|^2.
$
As for the second term,
\begin{align}
    \left |\frac{\rm{d}}{\rm{d}t}[\efl(\nu(t)) - \efl(\nu(0))] \right | &\le h \left |\iprod{\nabla_\theta  \efl(\nu(t)) - \nabla_\theta  \efl(\nu(0))}{\nabla_\theta \efl(\thetaf_n, \rf_n)}\right | \label{eq:discrete_t1}\\
    &+ h \left |\int \left (\delta_r \efl[\nu(t)] - \delta_r\efl[\nu(0)] \right )\nabla \cdot (\rf_{n} \nabla_z \delta_r \efl[\thetaf_n, \rf_n]))\, \rm{d}z \right | \label{eq:discrete_t2}
\end{align}
Focusing on the  RHS on \Cref{eq:discrete_t1} we have
\begin{align*}
    \text{RHS of \Cref{eq:discrete_t1}} &\le h\|\nabla_\theta \efl(\thetaf_n, \rf_n)\|\|\nabla_\theta  \efl(\nu(t)) - \nabla_\theta  \efl(\nu(t'))\| \\
    &\le K_{\cal{E}^\fudge_\lambda}h\|\nabla_\theta \efl(\thetaf_n, \rf_n)\| (\|\thetaf_{n+t} - \thetaf_{n}\| + \sf{W}_2(\rf_{n+t} , \rf_{n})),
\end{align*}
where we use Cauchy-Swharz for the first inequality; and for the second,  Lipschitz gradient property from \Cref{prop:lip_theta_grad_energy}. Using the following facts:
\begin{align*}
\|\thetaf_{n+t} - \thetaf_{n+t'}\| &= h |t-t'|\|\nabla_\theta \efl(\thetaf_n, \rf_n)\|,  \\
\sf{W}_2(\rf_{n+t} , \rf_{n+t'}) &\le h|t-t'|(\mathbb{E}_{\rf_n}\|\nabla_z \delta_r \efl[\thetaf_n, \rf_n]\|^2)^\frac{1}{2},
\end{align*}
with Young's inequality, we obtain
\begin{align}
    \text{RHS of \Cref{eq:discrete_t1}} &\le h^2K_{\cal{E}^\fudge_\lambda} |t-t'|\left  (\frac{3}{2}\|\nabla_\theta \efl(\thetaf_n, \rf_n)\|^2 + \frac{1}{2} \mathbb{E}_{\rf_n}\|\nabla_z \delta_r \efl[\thetaf_n, \rf_n]\|^2 \right ) \label{eq:bound_discrete_t1}
\end{align}
Similarly, for \Cref{eq:discrete_t2}, we have
\begin{align}
    \text{ \Cref{eq:discrete_t2}} &=
    h \left |\iprod{\nabla_r\left (\delta_r \efl[\nu(t)] - \delta_r\efl[\nu(t')] \right )}{\nabla_z \delta_r \efl[\thetaf_n, \rf_n])}_{\rf_{n}} \right |\nonumber \\
    &\le hK \left [ \|\thetaf_{n+t} - \thetaf_{n+t'}\| + \sf{W}_2(\rf_{n+t} , \rf_{n+t'}) \right ]\bb{E}\|\nabla_z \delta_r \efl[\thetaf_n, \rf_n])\| \nonumber\\
    &\le h^2 K|t-t'|\left (\frac{1}{2} \|\nabla_\theta \efl(\thetaf_n, \rf_n)\|^2 + \frac{3}{2} \bb{E}\|\nabla_z \delta_r \efl[\thetaf_n, \rf_n])\|^2\right ) \label{eq:bound_discrete_t2}
\end{align}
Thus, combining \Cref{eq:bound_discrete_t1} and \Cref{eq:bound_discrete_t2}, we otain
$$
\eqref{eq:bound_discrete_t1} + \eqref{eq:bound_discrete_t2} \le -h^2K|t-t'|2\|\nabla \efl(\thetaf_n, \rf_n)\|^2
$$
into \Cref{eq:desired_result}, we obtain
$$
\efl(\nu(1)) - \efl(\nu(0)) \le - h\left (1 - \frac{2Kh}{2} \right) \|\nabla_\cal{M} \efl(\thetaf_n, \rf_n)\|^2
$$
Hence, it is decreasing if $h < \frac{2}{K}$.
\end{proof}
