# Supplementary material for: Particle Semi-Implicit Variational Inference
Source: arXiv:2407.00649 source file (2025-01-14)
Supplement: Supplementary file 3 [file g-convergence.tex]

\documentclass[main]{subfiles}

\newcommand{\mSpace}{\mathcal{X}}

\begin{document}

\section{$\Gamma$-Convergence}

In this section, we will restate the results on $\Gamma$-convergence for completeness. For the details and proofs, we refer to \citep{dal2012introduction}. We shall assume that $\cal{X}$ is a metric space.
\begin{definition}[Coercive function]
    \label{def:coercive}
    A function $f:\mSpace \rightarrow \mathbb{R}$ is \textit{coercive} if for all $t \in \mathbb{R}$, the preimage $f^{-1}((-\infty, t]) = \{x\in \mSpace: f(x) = t\}$ is relatively compact.
\end{definition}
\begin{definition}[$\Gamma$-convergence]
	We say that a sequence $f_j:X \rightarrow \bb{R}$ $\Gamma$-converges to $f_\infty$, denoted by $f_\infty = \glim_j f_j$, if for all $x\in X$, we have
	\begin{itemize}
		\item (lim inf inequality) for every sequence $(x_j)$ converging to $x$,
		$$
		f_\infty (x) \le \liminf_j f_j (x_j);
		$$
		\item (lim sup inequality or recovering sequence) there exists a sequence $(x_j)$ converging to $x$ such that 
		$$
		f_\infty(x) \ge \limsup_j f_j (x_j).
		$$
	\end{itemize}
\end{definition}
\end{document}
